# Supplementary material for: Requirements Practices and Gaps When Engineering Human-Centered Artificial Intelligence Systems
Source: arXiv:2301.10404 source file (2023-01-25)
Supplement: Supplementary file 1 [file Appendix.tex]

\textbf{Area\#1} - User Needs: Which of the following aspects of user needs do you capture during early stages of building AI systems? (You can select more than one option) \\
\ding{111}	Identify the users of the system  \\
\ding{111}	Identify why the system is needed  \\
\ding{111}	Understand what the user expects from the system  \\
\ding{111}	Decide on the feasibility of AI as a solution to some of these needs (use a non-AI solution instead)\\
\ding{111}	Specify whether the AI will be used for augmenting (assisting the user) or automation (automating the task for users)   \\
\ding{111}	Determine if the end-user needs to be aware of the AI feature used in the system or not\\
\ding{111}	Determine if the AI features interact with the user without requesting (proactive), vs reacts to the users request or interaction (reactive) \\
\ding{111}	Specify the trade-offs between the ‘right’ and ‘wrong’ predictions? i.e., precision vs recall\\
\ding{111}	Specify how to monitor the reward function values over time - i.e. when the Machine Learning model might need to be re-trained  \\ 
\ding{111}	Our projects do not specify any user needs in the Requirements Engineering stage\\
\ding{111}	Other user needs that you identify in the Requirements Engineering stage?  \_\_\_\_\_\_ \\

\textbf{Area\#2} - Model requirements: Which of the following model needs do you specify when building AI systems? (You can select more than one option)\\
\ding{111}	Specify what the algorithm should optimize for?  (e.g. explainability, accuracy, robust)\\
\ding{111}	If using Machine Learning, specify what task should be used (e.g. regression, classification, clustering)\\
\ding{111}	 Specify which training method to use?  Dynamic (improves and learns form user feedback/behaviour) or static (trained offline, and only improves with updates)\\
\ding{111}	Specify how to balance between overfitting and underfitting \\
\ding{111}	Specify how to evaluate the model and which tools to use   \\
\ding{111}	Specify the execution time or scalability issues  \\
\ding{111}  Specify how user feedback is used in model tuning \\
\ding{111}	Specify how training data is used in model tuning \\
\ding{111}	Our projects do not specify any model requirements in the Requirements Engineering stage\\
\ding{111}	Other model requirements you would specify in the Requirements Engineering stage?   \\

\textbf{Area\#3} - Data requirements: What data requirements do you consider when building AI systems? (You can select more than one option)\\
\ding{111}	Specify what data sources and datasets to use in model training and testing \\
\ding{111}	Specify how to split the dataset into training and testing sets  \\
\ding{111}	Specify the minimum number of samples required  \\ 
\ding{111}	Sampling rate (Number of samples collected over a specified timeframe)   \\
\ding{111}	Specify how to label the data  \\
\ding{111}	Specify the features to be present in the dataset   \\ 
\ding{111}	Ensure the accuracy, coverage and correctness of data \\
\ding{111}	Ensure compliance with privacy and safety laws when collecting data  \\
\ding{111}	Avoid and mitigate biases in the data \\ 
\ding{111}	Design for incoming data from user feedback   \\
\ding{111}	Our projects do not specify any data requirements in the Requirements Engineering stage\\
\ding{111}	Other data requirements that you identify in the Requirements Engineering stage?\\ 

\textbf{Area\#4} - Feedback and User control:  Which of the following do you consider during the requirements engineering phase of AI systems? (You can select more than one option)\\
\ding{111}	Account for implicit feedback by monitoring users behaviours (e.g. the number of times they logged in, accepted/rejected recommendations)  \\
\ding{111}	Account for explicit feedback by asking the users to provide feedback (e.g rankings, thumbs up, ask user to input textual feedback)  \\
\ding{111}	Plan for explicit feedback by using surveys  \\ 
\ding{111}	Specify and insure data privacy of personal information when collecting feedback \\
\ding{111}	Specify how user feedback is used to improve model performance  \\
\ding{111}	Specify how user feedback is used in model tuning  \\ 
\ding{111}	Specify when the user should take control over the system or when action is required -- e.g. in a self-driving car   \\
\ding{111}	Specify when and how users can adjust their preferences  \\
\ding{111}	Our projects do not specify any feedback and user control needs in the Requirements Engineering stage \\ 
\ding{111}	Other requirements related to user feedback and control you would specify during RE\\ 

\textbf{Area\#5} - Explainability \& Trust: Which of the following explainability requirements do you consider when building Artificial Intelligence systems? (You can select more than one option) \\
\ding{111} Explain the limitations of the AI system to the end user   \\ 
\ding{111} Explain the systems functionalities to the end user  \\ 
\ding{111} Explain the data sources to the end user and that predictions are based on data  \\
\ding{111} Provide an explanation to the output and why these prediction values were given \\
\ding{111} Inform the user with any updates and changes done to the model or system   \\
\ding{111} Determine the level of detail needed to provide to the user -- i.e. provide just enough explanation based on which task the user is doing at the moment   \\
\ding{111} Explain consequences to users’ actions   \\
\ding{111} Accounting for explainability to conflict with other requirements such as performance, cost, development and security   \\
\ding{111} Avoid using predictions when confidence levels are low as it might create mistrust  \\ 
\ding{111} Do not provide an explanation, as it might be distracting or irrelevant   \\
\ding{111} Explain to the user how their information is used and shared (if any) with other vendors to avoid mistrust   \\
\ding{111} Our projects do not specify any explainability requirements in the Requirements Engineering  stage   \\
\ding{111} Other explainability requirements you would specify during the Requirements Engineering stage \\
 \\ 
\textbf{Area\#6} - Errors and graceful failures: Which of the following would you specify during the requirements phase when building AI systems? (You can select more than one option)\\ 
\ding{111}	Specify errors that might appear such as contexts, system and background errors   \\
\ding{111}	Specify error sources that might occur such as models, data and user input \\
\ding{111}	Gather feedback to why users continue to reject predictions  \\ 
\ding{111}	Avoid errors and incorrect assumptions that are made based on sensitive or private data  \\
\ding{111}	Allow users to fix mistakes\\
\ding{111}	Lookout for abusive users  \\ 
\ding{111}	Our projects do not specify how errors might occur or provide details of how to deal with failure in the RE stage   \\
\ding{111}	Other requirements for errors and graceful failures you might specify in the Requirements Engineering stage  \\
